# Supplementary material for: Multi-region relaxed magnetohydrodynamics in plasmas with slowly changing boundaries --- resonant response of a plasma slab
Source: arXiv:1609.00930 ancillary file (2017-03-17)
Supplement: Supplementary file 1 [file MRxMHDSlab_RMP_arx2017EXT.pdf]

# Electronic Supplement to: Multi-region relaxed magnetohydrodynamics in plasmas with slowly changing boundaries — resonant response of a plasma slab

R. L. Dewar*
*Centre for Plasmas and Fluids, Research School of Physics & Engineering, The Australian National University, Canberra, ACT 2601, Australia*

S. R. Hudson† and A. Bhattacharjee‡
*Princeton Plasma Physics Laboratory, PO Box 451, Princeton NJ 08543, USA*

Z. Yoshida§
*Graduate School of Frontier Sciences, University of Tokyo, Kashiwa, Chiba 277-8561, Japan*
(Dated: March 16 2017)

Provides extended versions of some equations in the main paper to show more steps in their derivations, plus an Appendix C (not in the main paper) providing an alternative, variational, derivation of the Grad–Shafranov form of the Beltrami equation.

## I. INTRODUCTION

The extended equations are: Eq. (46), Eq. (58), Eq. (66), Eq. (74), Eq. (A6), and Eqs. (B5–B7).

Appendix C also adds a derivation of the Grad–Shafranov form of the Beltrami equation, alternative to that given in Sec. III B, by deriving it directly from the Woltjer–Taylor variational principle of extremizing magnetic energy subject to the constraint of constant magnetic helicity.

## II. THE DYNAMICAL MRXMHD MODEL

## III. HKT-BELTRAMI SLAB MODEL

### A. Unperturbed pseudo-toroidal equilibrium

### B. Grad–Shafranov (GS) representation

### C. Fluxes

### D. Unperturbed state in GS representation

$$
\begin{aligned}
\psi_a &= \frac{2\sin^2(\mu_0 a/2)}{\mu_0}\frac{B_a}{2\sin(\mu_0 a/2)\cos(\mu_0 a/2)} \\
&= \frac{B_a}{\mu_0}\tan\frac{\mu_0 a}{2}\ ,
\end{aligned} \tag{46}
$$

## IV. RIPPLED STATES IN GS REPRESENTATION

### A. Rippled boundary conditions

### B. GS equation boundary conditions

### C. Unperturbed state: include only $k_y = 0$

$$
\begin{aligned}
\overline{\psi}_0 &= \frac{B_0}{a}\int_0^a dx\,\frac{1}{\mu_0}(1-\cos\mu_0 x) \\
&= \frac{B_0}{\mu_0}\left(1-\langle\cos\mu_0 x\rangle_0\right) \\
&\sim \frac{B_0}{\mu_0}\left[\frac{\mu_0^2 a^2}{6}+O(\mu_0^4)\right]\ ,
\end{aligned} \tag{58}
$$

where $\langle\cos\mu_0 x\rangle_0$ is defined in Eq. (40).

### D. Rippled state: include $k_y \neq 0$ terms

## V. ENERGY AND HELICITY IN GS REPRESENTATION

$$
\begin{aligned}
\mathcal{W}_\Sigma &= \frac{1}{2}\left\langle|\boldsymbol{\nabla}\widetilde{\psi}|^2+\mu^2\widetilde{\psi}^2\right\rangle \\
&= \frac{1}{2}\left(\left\langle\boldsymbol{\nabla}\cdot(\widetilde{\psi}\boldsymbol{\nabla}\widetilde{\psi})\right\rangle-\left\langle\widetilde{\psi}\nabla^2\widetilde{\psi}\right\rangle+\mu^2\left\langle\widetilde{\psi}^2\right\rangle\right) \\
&= \frac{1}{2}\widetilde{\psi}_{\rm bdy}\left\langle\nabla^2\widetilde{\psi}\right\rangle+\mu^2\left\langle\widetilde{\psi}^2\right\rangle \\
&= \frac{1}{2}(\psi_a-\overline{\psi})\mu\overline{F}+\frac{\psi_a-\psi_{\rm cut}}{2a\lambda_m}J_+ +\mu^2\left\langle\widetilde{\psi}^2\right\rangle\ ,
\end{aligned} \tag{66}
$$

* robert.dewar@anu.edu.au
† shudson@pppl.gov
‡ abhattac@pppl.gov
§ yoshida@ppl.k.u-tokyo.ac.jp

### A. Relative magnetic helicity

$$
\begin{aligned}
\mathcal{K} &\equiv \frac{\langle \mathbf{A}\cdot\mathbf{B}\rangle}{2} \\
&= \frac{\langle (\mathbf{B} - C\mathbf{e}_z)\cdot\mathbf{B}\rangle}{2\mu} \\
&= \frac{\mathcal{W}_\Sigma}{\mu} + \frac{\overline{F}^2}{2\mu} - \frac{\overline{F}C}{2\mu} \\
&= \frac{\mathcal{W}_\Sigma}{\mu} - \frac{\overline{\psi}\,\overline{F}}{2} \, ,
\end{aligned}
\tag{74}
$$

## VI. SHIELDED RMP SOLUTIONS

### A. HKT-like rippled boundary condition

### B. Sinusoidal rippled boundary condition

## VII. CONCLUSION

## APPENDICES

### Appendix A: Magnetic helicity conservation with moving boundaries

See main paper for full Appendix. Only the extended equation is given below:

$$
\begin{aligned}
2\mu_0\frac{dK}{dt} &= \int_{\partial\Omega} \mathbf{A}\cdot\mathbf{B}\,\mathbf{n}\cdot\mathbf{v}\,dS \\
&\quad + \int_\Omega \left[\frac{\partial\mathbf{A}}{\partial t}\cdot\mathbf{B} + \mathbf{A}\cdot\frac{\partial\mathbf{B}}{\partial t}\right] dV \\
&= \int_{\partial\Omega} \mathbf{n}\cdot\mathbf{v}\mathbf{A}\cdot\mathbf{B}\,dS \\
&\quad + \int_\Omega \left[\mathbf{B}\cdot\boldsymbol{\nabla}\varphi + \mathbf{A}\cdot\boldsymbol{\nabla}\times(\mathbf{v}\times\mathbf{B})\right] dV \\
&= \int_{\partial\Omega} \mathbf{n}\cdot\mathbf{v}\mathbf{A}\cdot\mathbf{B}\,dS \\
&\quad + \int_{\mathfrak{P}} \boldsymbol{\nabla}\cdot\left[\varphi\mathbf{B} + (\mathbf{v}\times\mathbf{B})\times\mathbf{A}\right] dV \\
&= \int_{\partial\mathfrak{P}} \mathbf{n}\cdot\left[\mathbf{v}\mathbf{A}\cdot\mathbf{B} + (\varphi + \mathbf{v}\cdot\mathbf{A})\mathbf{B} - \mathbf{v}\mathbf{A}\cdot\mathbf{B}\right] dS \\
&\quad + \sum_{l=1}^{\nu}\int_{S_l} \mathbf{n}\cdot\mathbf{B}\,[\![\varphi]\!]\,dS \\
&= \sum_{l=1}^{\nu}\int_{S_l} \mathbf{n}\cdot\mathbf{B}\,[\![\varphi]\!]\,dS
\end{aligned}
\tag{A6}
$$

where $\mathfrak{P}$ is the toroid $\Omega$ cut by $\nu$ topologically distinct surfaces of section $S_l$, $\mathbf{n}$ being the outward normal on $\partial\mathfrak{P}$. The jumps $[\![\varphi]\!]$ arise from the reversals of direction of $\mathbf{n}$ across the cuts.

### Appendix B: Vacuum Helicity

See main paper for full Appendix. Only the extended equations are given below:

$$
\begin{aligned}
K_+^{\rm H} &\equiv \int_{\Omega_+} \frac{\mathbf{A}^{\rm H}\cdot\mathbf{B}_{\rm H}}{2\mu_0}\,dV \\
&= \int_{\Omega_+} \frac{\left[-\psi^{\rm H}\mathbf{e}_z + \mathbf{e}_z\times\boldsymbol{\nabla}\left(\frac{1}{2}\overline{F}x^2\right)\right]\cdot(\overline{F}\,\mathbf{e}_z + \mathbf{e}_z\times\boldsymbol{\nabla}\psi^{\rm H})}{2\mu_0}\,dV \\
&= \int_{\Omega_i} \frac{\left[-\overline{F}\psi^{\rm H} + \mathbf{e}_z\times\boldsymbol{\nabla}\left(\frac{1}{2}\overline{F}x^2\right)\cdot(\mathbf{e}_z\times\boldsymbol{\nabla}\psi^{\rm H})\right]}{2\mu_0}\,dV \\
&= \int_{\Omega_+} \frac{\left[-\overline{F}\psi^{\rm H} + \left(\boldsymbol{\nabla}\frac{1}{2}\overline{F}x^2\right)\cdot\boldsymbol{\nabla}\psi^{\rm H})\right]}{2\mu_0}\,dV \, .
\end{aligned}
\tag{B5}
$$

Integration by parts then gives

$$
\begin{aligned}
K_+^{\rm H} &= \int_{\Omega_+} \frac{\left[-\overline{F}\psi^{\rm H} + \overline{F}\partial_x(x\psi^{\rm H})\right]}{2\mu_0}\,dV \\
&= \frac{\overline{F}}{2\mu_0}\left[-2\int_{\Omega_+}\psi^{\rm H}\,dV + \psi_a\int_{-\pi a}^{\pi a} x_{\rm bdy}(y)\,dy\right] \\
&= \frac{\overline{F}}{2\mu_0}\left[-2\int_{\Omega_+}\psi^{\rm H}\,dV + 2\pi a^2\psi_a\right] \, ,
\end{aligned}
\tag{B6}
$$

using the area constraint Eq. (37).

$$
\begin{aligned}
\int_{\Omega_+}\psi^{\rm H}\,dV &= \int_{\Omega_+}\Bigg(d_0^{\rm H}\,|x| \\
&\quad + \sum_{l=1}^{\infty} d_{lm}^{\rm H}\cos\frac{lmy}{a}\,\sinh\left|\frac{lmx}{a}\right|\Bigg)\,dV \\
&= \int_{-\pi a}^{\pi a} dy\,\Bigg[\frac{1}{2}d_0^{\rm H}x_{\rm bdy}^2(y) \\
&\quad + \sum_{l=1}^{\infty} d_{lm}^{\rm H}\cos\left(\frac{lmy}{a}\right)\left(\cosh\left|\frac{lmx_{\rm bdy}(y)}{a}\right| - 1\right)\Bigg] \, ,
\end{aligned}
\tag{B7}
$$

### Appendix C: Scalar Variational Principle

We use as a trial function for the vector potential

$$
\mathbf{A} = -\psi\boldsymbol{\nabla}z + G\boldsymbol{\nabla}Y \, , \tag{C1}
$$

giving a Clebsch representation of the magnetic field as the sum of orthogonal poloidal and toroidal components,

$$\mathbf{B} = \mathbf{B}_{\rm pol} + \mathbf{B}_{\rm tor} \ , \tag{C2a}$$
$$\mathbf{B}_{\rm pol} \equiv \boldsymbol{\nabla} z \times \boldsymbol{\nabla}\psi \ , \tag{C2b}$$
$$\mathbf{B}_{\rm tor} \equiv \boldsymbol{\nabla} G \times \boldsymbol{\nabla} Y \ . \tag{C2c}$$

In the above $\psi(x,y)$ is a poloidal flux function and $Y(x,y)$ is a generalized poloidal coordinate such that $Y(x,y) - y$ is a periodic function of $y$ (periodicity length $2\pi a$). Thus the pair $\psi, Y$ forms a curvilinear coordinate system in the $x, y$ plane (though with topological complications at island separatrices), the Jacobian of the transformation from $x, y$ to $\psi, Y$ being $\boldsymbol{\nabla}\psi \times \boldsymbol{\nabla} Y \boldsymbol{\cdot} \boldsymbol{\nabla} z$. In order that $\mathbf{B}\boldsymbol{\cdot}\boldsymbol{\nabla}\psi = 0$, so that level surfaces $\psi = \text{const}$ define magnetic surfaces, we constrain $G$ to depend only on $\psi$ by representing it as the function $G(\psi)$.

Relations between the as-yet-unknown scalar functions $\psi, Y, G$ are to be determined as Euler–Lagrange equations arising from the Woltjer–Taylor variational principle that the functional $I[\psi, Y, G]$ be stationary in a relaxed plasma under arbitrary variations $\delta\psi, \delta Y, \delta G$, where

$$I \equiv -\frac{1}{2}\iint_\Omega (B^2 - \mu\mathbf{A}\boldsymbol{\cdot}\mathbf{B})\, dA \ , \tag{C3}$$

$\Omega$ here being the two-dimensional cross section of the relaxed plasma domain in question [e.g. $y \in (0, 2\pi a)$, $x \in (0, x_{\rm bdy}(y))$] and $dA$ the element of area, $dxdy$. As in Sec. II $\mu$ is a Lagrange multiplier used to restrict variations of the magnetic energy to directions where the magnetic helicity is conserved.

Writing $\mathbf{B}_{\rm tor} = B_z\boldsymbol{\nabla} z$ we see from Eq. (C2c) that $B_z = \{G, Y\} = G'(\psi)\{\psi, Y\}$, the *Poisson bracket* $\{\cdot,\cdot\}$ between any functions $f$ and $g$ being defined as

$$\begin{aligned}\{f, g\} &\equiv \boldsymbol{\nabla} f \times \boldsymbol{\nabla} g \boldsymbol{\cdot} \boldsymbol{\nabla} z \\ &= \frac{\partial f}{\partial x}\frac{\partial g}{\partial y} - \frac{\partial g}{\partial x}\frac{\partial f}{\partial y} \\ &= \frac{\partial}{\partial x}\left(f\frac{\partial g}{\partial y}\right) - \frac{\partial}{\partial y}\left(f\frac{\partial g}{\partial x}\right)\end{aligned} \tag{C4}$$

the latter form being useful for integration by parts:

$$\begin{aligned}\{f, g\}h &\equiv \frac{\partial}{\partial x}\left(f\frac{\partial g}{\partial y}\right)h - \frac{\partial}{\partial y}\left(f\frac{\partial g}{\partial x}\right)h \\ &= f\{g, h\} \\ &\quad + \frac{\partial}{\partial x}\left(fh\frac{\partial g}{\partial y}\right) - \frac{\partial}{\partial y}\left(fh\frac{\partial g}{\partial x}\right) \ .\end{aligned} \tag{C5}$$

From Eq. (C2b) and Eq. (C2c) we have

$$B^2_{\rm pol} = |\boldsymbol{\nabla}\psi|^2 \ , \tag{C6a}$$
$$B^2_{\rm tor} = \{G, Y\}^2 \ . \tag{C6b}$$

and, using Eq. (C1) and Eq. (C2a), we also have

$$\mathbf{A}\boldsymbol{\cdot}\mathbf{B} = \{\psi, Y\}G - \{G, Y\}\psi \tag{C7}$$

Thus Eq. (C3) becomes

$$\begin{aligned}I = \frac{1}{2}\iint_\Omega \Big(&-|\boldsymbol{\nabla}\psi|^2 - \{G, Y\}^2 \\ &+ \mu G\{\psi, Y\} - \mu\psi\{G, Y\}\Big)\, dA \ ,\end{aligned} \tag{C8}$$

Restricting to variations internal to the domain $\Omega$, we can integrate by parts using the identity Eq. (C5) without worrying about surface variations. Denoting by $\delta_Y f$ variations in any functional $f[\psi, Y, G]$ induced by $\delta Y$, the $Y$-variation in $I$ is

$$\begin{aligned}\delta_Y I &= \frac{1}{2}\iint_\Omega \Big(-2\{G, \delta Y\}\{G, Y\} \\ &\qquad + \mu G\{\psi, \delta Y\} - \mu\psi\{G, \delta Y\}\Big)\, dA \\ &= \iint_\Omega \Big(\{G, \{G, Y\}\} + \mu\{G, \psi\}\Big)\, \delta Y\, dA \ .\end{aligned} \tag{C9}$$

Setting the coefficient of the arbitrary variation $\delta Y$ to zero, noting that $\{G, \psi\} \equiv G'\{\psi, \psi\} = 0$, we find the Euler–Lagrange equation

$$G'\left\{\psi, \{G, Y\}\right\} = 0 \ . \tag{C10}$$

Assuming $G' \neq 0$, this implies $\{G, Y\}$ *is a function (F, say) of $\psi$ alone*,

$$\{G, Y\} = F(\psi) \ . \tag{C11}$$

As noted above, $\{G, Y\} = B_z$, so we have thus shown the equivalence of Eq. (C2a) and Eq. (19)

The corresponding variation induced by $\delta\psi$ is

$$\begin{aligned}\delta_\psi I &= \frac{1}{2}\iint_\Omega \Big(-2\boldsymbol{\nabla}\psi\boldsymbol{\cdot}\boldsymbol{\nabla}\delta\psi - 2\{\delta_\psi G, Y\}\{G, Y\} \\ &\qquad + \mu G\{\delta\psi, Y\} + \mu\delta_\psi G\{\psi, Y\} \\ &\qquad - \mu\delta\psi\{G, Y\} - \mu\psi\{\delta_\psi G, Y\}\Big)\, dA \\ &= \iint_\Omega \Big(\nabla^2\psi + G'\{\{G, Y\}, Y\} \\ &\qquad + \mu G'\{\psi, Y\} - \mu\{G, Y\}\Big)\, \delta\psi\, dA\end{aligned} \tag{C12}$$

where $\delta_\psi G = G'\delta\psi$.

Noting that the last two terms in the coefficient of $\delta\psi$ cancel, we find our second Euler–Lagrange equation,

$$\boldsymbol{\nabla}^2\psi + G'\left\{\{G, Y\},\ Y\right\} = 0 \ . \tag{C13}$$

Using Eq. (C11) we have $G'\left\{\{G, Y\},\ Y\right\} = G'F'\{\psi, Y\} = FF'$, showing the equivalence of Eq. (C13) and the Grad–Shafranov equation Eq. (22).

Finally, consider variations in the functional form of

$G(\psi)$,

$$\begin{aligned}\delta_G I &= \frac{1}{2}\iint_\Omega \Big(-2\{\delta G, Y\}\{G, Y\} \\ &\qquad + \mu\delta G\{\psi, Y\} - \mu\psi\{\delta G, Y\}\Big)\, dA \\ &= \iint_\Omega \Big(\{\{G, Y\},\ Y\} + \mu\{\psi, Y\}\Big)\,\delta G\, dA \\ &= \iint_\Omega [F'(\psi) + \mu]\delta G(\psi)\,\{\psi, Y\} dA\ ,\end{aligned} \tag{C14}$$

where we used Eq. (C11) to show that the coefficient of $\delta G(\psi)$ is also a function only of $\psi$. Noting that $\{\psi, Y\}dA = d\psi dY$ we see that our third Euler–Lagrange equation is

$$F'(\psi) + \mu = 0\ , \tag{C15}$$

which agrees with eq. (24), thus completing our variational derivation of the Grad–Shafranov form of the Beltrami equation.
